# Supplementary material for: On the mathematical structure of quantum models of computation based on Hamiltonian minimisation
Source: arXiv:2009.10088 source file (2021-12-24)
Supplement: Supplementary file 1 [file appendix.tex]

\appendix
%% Правка оформления ссылок на приложения:
%http://tex.stackexchange.com/questions/56839/chaptername-is-used-even-for-appendix-chapters-in-toc
%http://tex.stackexchange.com/questions/59349/table-of-contents-with-chapter-and-appendix
%% требует двойной компиляции
\addtocontents{toc}{\def\protect\cftchappresnum{\appendixname{} }%
\setlength{\cftchapnumwidth}{\widthof{\cftchapfont\appendixname~Ш\cftchapaftersnum}}%
}
%% Оформление заголовков приложений ближе к ГОСТ:
\sectionformat{\chapter}[display]{% Параметры заголовков разделов в тексте
    label=\chaptertitlename\ \thechapter,% (ГОСТ Р 2.105, 4.3.6)
    labelsep=20pt,
}

% \appendix
% %% Правка оформления ссылок на приложения:
% %http://tex.stackexchange.com/questions/56839/chaptername-is-used-even-for-appendix-chapters-in-toc
% %http://tex.stackexchange.com/questions/59349/table-of-contents-with-chapter-and-appendix
% %% требует двойной компиляции
% \addtocontents{toc}{\def\protect\cftchappresnum{\appendixname{} }%
% \setlength{\cftchapnumwidth}{\widthof{\cftchapfont\appendixname~Ш\cftchapaftersnum}}%
% }
% %% Оформление заголовков приложений ближе к ГОСТ:
% \sectionformat{\chapter}[display]{% Параметры заголовков разделов в тексте
%     label=\chaptertitlename\ \thechapter,% (ГОСТ Р 2.105, 4.3.6)
%     labelsep=20pt,
% }
% % \renewcommand\thechapter{\Asbuk{chapter}} % Чтобы приложения русскими буквами нумеровались
   % Предварительные настройки для правильного подключения Приложений
\chapter{Примеры вставки листингов программного кода} \label{AppendixA}

Для крупных листингов есть два способа. Первый красивый, но в нём могут быть проблемы с поддержкой кириллицы (у вас может встречаться в комментариях и
печатаемых сообщениях), он представлен на листинге~\ref{list:hwbeauty}.
\begin{ListingEnv}[H]% буква H означает Here, ставим здесь,
    % элементы, которые нежелательно разрывать обычно не ставят
    % посреди страницы: вместо H используется t (top, сверху страницы),
    % или b (bottom) или p (page, на отдельной странице)
%    \captionsetup{format=tablenocaption}% должен стоять до самого caption
%    \thisfloatsetup{\capposition=top}%
    \caption{Программа “Hello, world” на \protect\cpp}
    % далее метка для ссылки:
    \label{list:hwbeauty}
    % окружение учитывает пробелы и табляции и приеняет их в сответсвии с настройкми
    \begin{lstlisting}[language={[ISO]C++}]
	#include <iostream>
	using namespace std;

	int main() //кириллица в комментариях при xelatex и lualatex имеет проблемы с пробелами
	{
		cout << "Hello, world" << endl; //latin letters in commentaries
		system("pause");
		return 0;
	}
    \end{lstlisting}
\end{ListingEnv}%
Второй не такой красивый, но без ограничений (см.~листинг~\ref{list:hwplain}).
\begin{ListingEnv}[H]
    \begin{Verb}
        
        #include <iostream>
        using namespace std;
        
        int main() //кириллица в комментариях
        {
            cout << "Привет, мир" << endl;
        }
    \end{Verb}
    \caption{Программа “Hello, world” без подсветки}
    \label{list:hwplain}
\end{ListingEnv}

Можно использовать первый для вставки небольших фрагментов
внутри текста, а второй для вставки полного
кода в приложении, если таковое имеется.

Если нужно вставить совсем короткий пример кода (одна или две строки), то выделение  линейками и нумерация может смотреться чересчур громоздко. В таких случаях можно использовать окружения \texttt{lstlisting} или \texttt{Verb} без \texttt{ListingEnv}. Приведём такой пример с указанием языка программирования, отличного от заданного по умолчанию:
\begin{lstlisting}[language=Haskell]
fibs = 0 : 1 : zipWith (+) fibs (tail fibs)
\end{lstlisting}
Такое решение~--- со вставкой нумерованных листингов покрупнее
и вставок без выделения для маленьких фрагментов~--- выбрано,
например, в книге Эндрю Таненбаума и Тодда Остина по архитектуре
%компьютера~\autocite{TanAus2013} (см.~рис.~\ref{fig:tan-aus}).

Наконец, для оформления идентификаторов внутри строк
(функция \lstinline{main} и тому подобное) используется
\texttt{lstinline} или, самое простое, моноширинный текст
(\texttt{\textbackslash texttt}).

Пример~\ref{list:internal3}, иллюстрирующий подключение переопределённого языка. Может быть полезным, если подсветка кода работает криво. Без дополнительного окружения, с подписью и ссылкой, реализованной встроенным средством.
\begin{lstlisting}[language={Renhanced},caption={Пример листинга c подписью собственными средствами},label={list:internal3}]
## Caching the Inverse of a Matrix

## Matrix inversion is usually a costly computation and there may be some
## benefit to caching the inverse of a matrix rather than compute it repeatedly
## This is a pair of functions that cache the inverse of a matrix.

## makeCacheMatrix creates a special "matrix" object that can cache its inverse

makeCacheMatrix <- function(x = matrix()) {#кириллица в комментариях при xelatex и lualatex имеет проблемы с пробелами
    i <- NULL
    set <- function(y) {
        x <<- y
        i <<- NULL
    }
    get <- function() x
    setSolved <- function(solve) i <<- solve
    getSolved <- function() i
    list(set = set, get = get,
    setSolved = setSolved,
    getSolved = getSolved)
    
}


## cacheSolve computes the inverse of the special "matrix" returned by
## makeCacheMatrix above. If the inverse has already been calculated (and the
## matrix has not changed), then the cachesolve should retrieve the inverse from
## the cache.

cacheSolve <- function(x, ...) {
    ## Return a matrix that is the inverse of 'x'
    i <- x$getSolved()
    if(!is.null(i)) {
        message("getting cached data")
        return(i)
    }
    data <- x$get()
    i <- solve(data, ...)
    x$setSolved(i)
    i  
}
\end{lstlisting} %$ %Комментарий для корректной подсветки синтаксиса
                 %вне листинга

Листинг~\ref{list:external1} подгружается из внешнего файла. Приходится загружать без окружения дополнительного. Иначе по страницам не переносится.
    \lstinputlisting[lastline=78,language={R},caption={Листинг из внешнего файла},label={list:external1}]{listings/run_analysis.R}

\chapter{Очень длинное название второго приложения, в котором продемонстрирована работа с длинными таблицами} \label{AppendixB}

 \section{Подраздел приложения}\label{AppendixB1}
Вот размещается длинная таблица:
\fontsize{10pt}{10pt}\selectfont
\begin{longtable}[c]{|l|c|l|l|}
% \caption{Описание входных файлов модели}\label{Namelists} 
%\\ 
 \hline
 %\multicolumn{4}{|c|}{\textbf{Файл puma\_namelist}}        \\ \hline
 Параметр & Умолч. & Тип & Описание               \\ \hline
                                              \endfirsthead   \hline
 \multicolumn{4}{|c|}{\small\slshape (продолжение)}        \\ \hline
 Параметр & Умолч. & Тип & Описание               \\ \hline
                                              \endhead        \hline
% \multicolumn{4}{|c|}{\small\slshape (окончание)}        \\ \hline
% Параметр & Умолч. & Тип & Описание               \\ \hline
%                                             \endlasthead        \hline
 \multicolumn{4}{|r|}{\small\slshape продолжение следует}  \\ \hline
                                              \endfoot        \hline
                                              \endlastfoot
 \multicolumn{4}{|l|}{\&INP}        \\ \hline 
 kick & 1 & int & 0: инициализация без шума ($p_s = const$) \\
      &   &     & 1: генерация белого шума                  \\
      &   &     & 2: генерация белого шума симметрично относительно \\
  & & & экватора    \\
 mars & 0 & int & 1: инициализация модели для планеты Марс     \\
 kick & 1 & int & 0: инициализация без шума ($p_s = const$) \\
      &   &     & 1: генерация белого шума                  \\
      &   &     & 2: генерация белого шума симметрично относительно \\
  & & & экватора    \\
 mars & 0 & int & 1: инициализация модели для планеты Марс     \\
kick & 1 & int & 0: инициализация без шума ($p_s = const$) \\
      &   &     & 1: генерация белого шума                  \\
      &   &     & 2: генерация белого шума симметрично относительно \\
  & & & экватора    \\
 mars & 0 & int & 1: инициализация модели для планеты Марс     \\
kick & 1 & int & 0: инициализация без шума ($p_s = const$) \\
      &   &     & 1: генерация белого шума                  \\
      &   &     & 2: генерация белого шума симметрично относительно \\
  & & & экватора    \\
 mars & 0 & int & 1: инициализация модели для планеты Марс     \\
kick & 1 & int & 0: инициализация без шума ($p_s = const$) \\
      &   &     & 1: генерация белого шума                  \\
      &   &     & 2: генерация белого шума симметрично относительно \\
  & & & экватора    \\
 mars & 0 & int & 1: инициализация модели для планеты Марс     \\
kick & 1 & int & 0: инициализация без шума ($p_s = const$) \\
      &   &     & 1: генерация белого шума                  \\
      &   &     & 2: генерация белого шума симметрично относительно \\
  & & & экватора    \\
 mars & 0 & int & 1: инициализация модели для планеты Марс     \\
kick & 1 & int & 0: инициализация без шума ($p_s = const$) \\
      &   &     & 1: генерация белого шума                  \\
      &   &     & 2: генерация белого шума симметрично относительно \\
  & & & экватора    \\
 mars & 0 & int & 1: инициализация модели для планеты Марс     \\
kick & 1 & int & 0: инициализация без шума ($p_s = const$) \\
      &   &     & 1: генерация белого шума                  \\
      &   &     & 2: генерация белого шума симметрично относительно \\
  & & & экватора    \\
 mars & 0 & int & 1: инициализация модели для планеты Марс     \\
kick & 1 & int & 0: инициализация без шума ($p_s = const$) \\
      &   &     & 1: генерация белого шума                  \\
      &   &     & 2: генерация белого шума симметрично относительно \\
  & & & экватора    \\
 mars & 0 & int & 1: инициализация модели для планеты Марс     \\
kick & 1 & int & 0: инициализация без шума ($p_s = const$) \\
      &   &     & 1: генерация белого шума                  \\
      &   &     & 2: генерация белого шума симметрично относительно \\
  & & & экватора    \\
 mars & 0 & int & 1: инициализация модели для планеты Марс     \\
kick & 1 & int & 0: инициализация без шума ($p_s = const$) \\
      &   &     & 1: генерация белого шума                  \\
      &   &     & 2: генерация белого шума симметрично относительно \\
  & & & экватора    \\
 mars & 0 & int & 1: инициализация модели для планеты Марс     \\
kick & 1 & int & 0: инициализация без шума ($p_s = const$) \\
      &   &     & 1: генерация белого шума                  \\
      &   &     & 2: генерация белого шума симметрично относительно \\
  & & & экватора    \\
 mars & 0 & int & 1: инициализация модели для планеты Марс     \\
kick & 1 & int & 0: инициализация без шума ($p_s = const$) \\
      &   &     & 1: генерация белого шума                  \\
      &   &     & 2: генерация белого шума симметрично относительно \\
  & & & экватора    \\
 mars & 0 & int & 1: инициализация модели для планеты Марс     \\
kick & 1 & int & 0: инициализация без шума ($p_s = const$) \\
      &   &     & 1: генерация белого шума                  \\
      &   &     & 2: генерация белого шума симметрично относительно \\
  & & & экватора    \\
 mars & 0 & int & 1: инициализация модели для планеты Марс     \\
kick & 1 & int & 0: инициализация без шума ($p_s = const$) \\
      &   &     & 1: генерация белого шума                  \\
      &   &     & 2: генерация белого шума симметрично относительно \\
  & & & экватора    \\
 mars & 0 & int & 1: инициализация модели для планеты Марс     \\
 \hline
  %& & & $\:$ \\ 
 \multicolumn{4}{|l|}{\&SURFPAR}        \\ \hline
kick & 1 & int & 0: инициализация без шума ($p_s = const$) \\
      &   &     & 1: генерация белого шума                  \\
      &   &     & 2: генерация белого шума симметрично относительно \\
  & & & экватора    \\
 mars & 0 & int & 1: инициализация модели для планеты Марс     \\
kick & 1 & int & 0: инициализация без шума ($p_s = const$) \\
      &   &     & 1: генерация белого шума                  \\
      &   &     & 2: генерация белого шума симметрично относительно \\
  & & & экватора    \\
 mars & 0 & int & 1: инициализация модели для планеты Марс     \\
kick & 1 & int & 0: инициализация без шума ($p_s = const$) \\
      &   &     & 1: генерация белого шума                  \\
      &   &     & 2: генерация белого шума симметрично относительно \\
  & & & экватора    \\
 mars & 0 & int & 1: инициализация модели для планеты Марс     \\
kick & 1 & int & 0: инициализация без шума ($p_s = const$) \\
      &   &     & 1: генерация белого шума                  \\
      &   &     & 2: генерация белого шума симметрично относительно \\
  & & & экватора    \\
 mars & 0 & int & 1: инициализация модели для планеты Марс     \\
kick & 1 & int & 0: инициализация без шума ($p_s = const$) \\
      &   &     & 1: генерация белого шума                  \\
      &   &     & 2: генерация белого шума симметрично относительно \\
  & & & экватора    \\
 mars & 0 & int & 1: инициализация модели для планеты Марс     \\
kick & 1 & int & 0: инициализация без шума ($p_s = const$) \\
      &   &     & 1: генерация белого шума                  \\
      &   &     & 2: генерация белого шума симметрично относительно \\
  & & & экватора    \\
 mars & 0 & int & 1: инициализация модели для планеты Марс     \\
kick & 1 & int & 0: инициализация без шума ($p_s = const$) \\
      &   &     & 1: генерация белого шума                  \\
      &   &     & 2: генерация белого шума симметрично относительно \\
  & & & экватора    \\
 mars & 0 & int & 1: инициализация модели для планеты Марс     \\
kick & 1 & int & 0: инициализация без шума ($p_s = const$) \\
      &   &     & 1: генерация белого шума                  \\
      &   &     & 2: генерация белого шума симметрично относительно \\
  & & & экватора    \\
 mars & 0 & int & 1: инициализация модели для планеты Марс     \\
kick & 1 & int & 0: инициализация без шума ($p_s = const$) \\
      &   &     & 1: генерация белого шума                  \\
      &   &     & 2: генерация белого шума симметрично относительно \\
  & & & экватора    \\
 mars & 0 & int & 1: инициализация модели для планеты Марс     \\ 
 \hline 
\end{longtable}

\normalsize% возвращаем шрифт к нормальному
\section{Ещё один подраздел приложения} \label{AppendixB2}

Нужно больше подразделов приложения!

Пример длинной таблицы с записью продолжения по ГОСТ 2.105

    \centering
	\small
    \begin{longtable}[c]{|l|c|l|l|}
	\caption{Наименование таблицы средней длины}%
    \label{tbl:test5}% label всегда желательно идти после caption
    \\
    \hline
     %\multicolumn{4}{|c|}{\textbf{Файл puma\_namelist}}        \\ \hline
     Параметр & Умолч. & Тип & Описание\\ \hline
     \endfirsthead%
%     \multicolumn{4}{|c|}{\small\slshape (продолжение)}        \\ \hline
 \captionsetup{format=tablenocaption,labelformat=continued}% должен стоять до самого caption
    \caption[]{}\\
    \hline
     Параметр & Умолч. & Тип & Описание\\ \hline
      \endhead
      \hline
%     \multicolumn{4}{|r|}{\small\slshape продолжение следует}  \\
%\hline
     \endfoot
         \hline
     \endlastfoot
     \multicolumn{4}{|l|}{\&INP}        \\ \hline 
     kick & 1 & int & 0: инициализация без шума ($p_s = const$) \\
          &   &     & 1: генерация белого шума                  \\
          &   &     & 2: генерация белого шума симметрично относительно \\
      & & & экватора    \\
     mars & 0 & int & 1: инициализация модели для планеты Марс     \\
     kick & 1 & int & 0: инициализация без шума ($p_s = const$) \\
          &   &     & 1: генерация белого шума                  \\
          &   &     & 2: генерация белого шума симметрично относительно \\
      & & & экватора    \\
     mars & 0 & int & 1: инициализация модели для планеты Марс     \\
    kick & 1 & int & 0: инициализация без шума ($p_s = const$) \\
          &   &     & 1: генерация белого шума                  \\
          &   &     & 2: генерация белого шума симметрично относительно \\
      & & & экватора    \\
     mars & 0 & int & 1: инициализация модели для планеты Марс     \\
    kick & 1 & int & 0: инициализация без шума ($p_s = const$) \\
          &   &     & 1: генерация белого шума                  \\
          &   &     & 2: генерация белого шума симметрично относительно \\
      & & & экватора    \\
     mars & 0 & int & 1: инициализация модели для планеты Марс     \\
    kick & 1 & int & 0: инициализация без шума ($p_s = const$) \\
          &   &     & 1: генерация белого шума                  \\
          &   &     & 2: генерация белого шума симметрично относительно \\
      & & & экватора    \\
     mars & 0 & int & 1: инициализация модели для планеты Марс     \\
    kick & 1 & int & 0: инициализация без шума ($p_s = const$) \\
          &   &     & 1: генерация белого шума                  \\
          &   &     & 2: генерация белого шума симметрично относительно \\
      & & & экватора    \\
     mars & 0 & int & 1: инициализация модели для планеты Марс     \\
    kick & 1 & int & 0: инициализация без шума ($p_s = const$) \\
          &   &     & 1: генерация белого шума                  \\
          &   &     & 2: генерация белого шума симметрично относительно \\
      & & & экватора    \\
     mars & 0 & int & 1: инициализация модели для планеты Марс     \\
    kick & 1 & int & 0: инициализация без шума ($p_s = const$) \\
          &   &     & 1: генерация белого шума                  \\
          &   &     & 2: генерация белого шума симметрично относительно \\
      & & & экватора    \\
     mars & 0 & int & 1: инициализация модели для планеты Марс     \\
    kick & 1 & int & 0: инициализация без шума ($p_s = const$) \\
          &   &     & 1: генерация белого шума                  \\
          &   &     & 2: генерация белого шума симметрично относительно \\
      & & & экватора    \\
     mars & 0 & int & 1: инициализация модели для планеты Марс     \\
    kick & 1 & int & 0: инициализация без шума ($p_s = const$) \\
          &   &     & 1: генерация белого шума                  \\
          &   &     & 2: генерация белого шума симметрично относительно \\
      & & & экватора    \\
     mars & 0 & int & 1: инициализация модели для планеты Марс     \\
    kick & 1 & int & 0: инициализация без шума ($p_s = const$) \\
          &   &     & 1: генерация белого шума                  \\
          &   &     & 2: генерация белого шума симметрично относительно \\
      & & & экватора    \\
     mars & 0 & int & 1: инициализация модели для планеты Марс     \\
    kick & 1 & int & 0: инициализация без шума ($p_s = const$) \\
          &   &     & 1: генерация белого шума                  \\
          &   &     & 2: генерация белого шума симметрично относительно \\
      & & & экватора    \\
     mars & 0 & int & 1: инициализация модели для планеты Марс     \\
    kick & 1 & int & 0: инициализация без шума ($p_s = const$) \\
          &   &     & 1: генерация белого шума                  \\
          &   &     & 2: генерация белого шума симметрично относительно \\
      & & & экватора    \\
     mars & 0 & int & 1: инициализация модели для планеты Марс     \\
    kick & 1 & int & 0: инициализация без шума ($p_s = const$) \\
          &   &     & 1: генерация белого шума                  \\
          &   &     & 2: генерация белого шума симметрично относительно \\
      & & & экватора    \\
     mars & 0 & int & 1: инициализация модели для планеты Марс     \\
    kick & 1 & int & 0: инициализация без шума ($p_s = const$) \\
          &   &     & 1: генерация белого шума                  \\
          &   &     & 2: генерация белого шума симметрично относительно \\
      & & & экватора    \\
     mars & 0 & int & 1: инициализация модели для планеты Марс     \\
     \hline
      %& & & $\:$ \\ 
     \multicolumn{4}{|l|}{\&SURFPAR}        \\ \hline
    kick & 1 & int & 0: инициализация без шума ($p_s = const$) \\
          &   &     & 1: генерация белого шума                  \\
          &   &     & 2: генерация белого шума симметрично относительно \\
      & & & экватора    \\
     mars & 0 & int & 1: инициализация модели для планеты Марс     \\
    kick & 1 & int & 0: инициализация без шума ($p_s = const$) \\
          &   &     & 1: генерация белого шума                  \\
          &   &     & 2: генерация белого шума симметрично относительно \\
      & & & экватора    \\
     mars & 0 & int & 1: инициализация модели для планеты Марс     \\
    kick & 1 & int & 0: инициализация без шума ($p_s = const$) \\
          &   &     & 1: генерация белого шума                  \\
          &   &     & 2: генерация белого шума симметрично относительно \\
      & & & экватора    \\
     mars & 0 & int & 1: инициализация модели для планеты Марс     \\
    kick & 1 & int & 0: инициализация без шума ($p_s = const$) \\
          &   &     & 1: генерация белого шума                  \\
          &   &     & 2: генерация белого шума симметрично относительно \\
      & & & экватора    \\
     mars & 0 & int & 1: инициализация модели для планеты Марс     \\
    kick & 1 & int & 0: инициализация без шума ($p_s = const$) \\
          &   &     & 1: генерация белого шума                  \\
          &   &     & 2: генерация белого шума симметрично относительно \\
      & & & экватора    \\
     mars & 0 & int & 1: инициализация модели для планеты Марс     \\
    kick & 1 & int & 0: инициализация без шума ($p_s = const$) \\
          &   &     & 1: генерация белого шума                  \\
          &   &     & 2: генерация белого шума симметрично относительно \\
      & & & экватора    \\
     mars & 0 & int & 1: инициализация модели для планеты Марс     \\
    kick & 1 & int & 0: инициализация без шума ($p_s = const$) \\
          &   &     & 1: генерация белого шума                  \\
          &   &     & 2: генерация белого шума симметрично относительно \\
      & & & экватора    \\
     mars & 0 & int & 1: инициализация модели для планеты Марс     \\
    kick & 1 & int & 0: инициализация без шума ($p_s = const$) \\
          &   &     & 1: генерация белого шума                  \\
          &   &     & 2: генерация белого шума симметрично относительно \\
      & & & экватора    \\
     mars & 0 & int & 1: инициализация модели для планеты Марс     \\
    kick & 1 & int & 0: инициализация без шума ($p_s = const$) \\
          &   &     & 1: генерация белого шума                  \\
          &   &     & 2: генерация белого шума симметрично относительно \\
      & & & экватора    \\
     mars & 0 & int & 1: инициализация модели для планеты Марс     \\ 
%     \hline 
    \end{longtable}
\normalsize% возвращаем шрифт к нормальному
\section{Очередной подраздел приложения} \label{AppendixB3}

Нужно больше подразделов приложения!

\section{И ещё один подраздел приложения} \label{AppendixB4}

Нужно больше подразделов приложения!
