# Supplementary material for: On the mathematical structure of quantum models of computation based on Hamiltonian minimisation
Source: arXiv:2009.10088 source file (2021-12-24)
Supplement: Supplementary file 2 [file appendixsetup.tex]

\appendix
%% Правка оформления ссылок на приложения:
%http://tex.stackexchange.com/questions/56839/chaptername-is-used-even-for-appendix-chapters-in-toc
%http://tex.stackexchange.com/questions/59349/table-of-contents-with-chapter-and-appendix
%% требует двойной компиляции
\addtocontents{toc}{\def\protect\cftchappresnum{\appendixname{} }%
\setlength{\cftchapnumwidth}{\widthof{\cftchapfont\appendixname~Ш\cftchapaftersnum}}%
}
%% Оформление заголовков приложений ближе к ГОСТ:
\sectionformat{\chapter}[display]{% Параметры заголовков разделов в тексте
    label=\chaptertitlename\ \thechapter,% (ГОСТ Р 2.105, 4.3.6)
    labelsep=20pt,
}

% \appendix
% %% Правка оформления ссылок на приложения:
% %http://tex.stackexchange.com/questions/56839/chaptername-is-used-even-for-appendix-chapters-in-toc
% %http://tex.stackexchange.com/questions/59349/table-of-contents-with-chapter-and-appendix
% %% требует двойной компиляции
% \addtocontents{toc}{\def\protect\cftchappresnum{\appendixname{} }%
% \setlength{\cftchapnumwidth}{\widthof{\cftchapfont\appendixname~Ш\cftchapaftersnum}}%
% }
% %% Оформление заголовков приложений ближе к ГОСТ:
% \sectionformat{\chapter}[display]{% Параметры заголовков разделов в тексте
%     label=\chaptertitlename\ \thechapter,% (ГОСТ Р 2.105, 4.3.6)
%     labelsep=20pt,
% }
% % \renewcommand\thechapter{\Asbuk{chapter}} % Чтобы приложения русскими буквами нумеровались
